# Supplementary material for: An evidence-guided reinforcement learning method to improve psychiatric reasoning in small language models
Source: arXiv:2602.06449 source file (2026-08-31)
Supplement: Supplementary file 1 [file appendix-prompt.tex]

\section*{Appendix A: Prompt Specifications for Dataset Curation and Evaluation}
This appendix details the exact prompts used to facilitate the dataset creation pipeline.
%---------------------------------------A.1------------------------------------------
\subsection*{A.1 Generation Prompts}
\vspace{0.5em}
The following prompts are used to generate content for various medical evaluation tasks.

\subsubsection*{A.1.1 Medical MCQ Generation Prompt}
\begin{tcolorbox}[colback=gray!5!white,colframe=gray!55!white,before upper={\raggedright},title=Medical MCQ Generation Prompt]
You are a senior clinical medical educator. Please carefully read the following psychiatric case report and generate 3 high-quality, independent multiple-choice questions (MCQs) to assess the clinical reasoning and medical knowledge abilities of AI systems.\\
\vspace{1em}
\textbf{Strict requirements:}\\
1. Each question must be fully independent and self-contained: The stem of each question must include all essential information needed to answer the question. (Ex, patient's age, gender, medical history, clinical course, relevant lab/imaging findings, treatment details, etc.) Do not omit, abbreviate or assume any information. Avoid phrases such as "this patient," "the above case," or "as previously described."

2. It is acceptable and necessary for different questions to repeat case details. Any form of inter-question dependency is strictly forbidden; each question must make sense and be answerable in complete isolation.

3. Each MCQ should have four medically plausible options (A-D), with only one correct answer.

4. Mark the correct answer as "A", and provide a concise professional explanation (≤100 words).

5. The questions should cover: the patient's clinical background, detailed medical events, underlying pathogenesis, diagnos are differential, laboratory \& imaging findings, therapy strategies, prognosis, etc. They should test deep clinical reasoning across complex, multi-faceted medical information.

6. Output only the following strict JSON format (content in English):

\begin{spacing}{1.0}
\begin{lstlisting}[breaklines=true, basicstyle=\ttfamily\normalsize]
[
  {
    "question": "Fully explicit stem: patient background, course, labs, imaging, treatment, etc. All necessary information for this question must be provided so it stands alone.",
    "options": {
      "A": "Correct answer (only one correct)",
      "B": "Distractor B",
      "C": "Distractor C",
      "D": "Distractor D"
    },
    "answer": "A",
    "explanation": "Concise clinical rationale (≤100 words)"
  },
  ...
]
\end{lstlisting}
\end{spacing}

Below is the full original case report (read thoroughly to generate the questions):

\{full article content\}
\end{tcolorbox}

%---------------------------------------A.2------------------------------------------
\newpage
\subsection*{A.2 Question-Type Screening Prompts}
\vspace{0.5em}
The following prompt is used to classify psychiatric questions using a two-step hierarchical approach based on ICD-11. The model is instructed to first identify the major diagnostic category, then select the most specific diagnosis from the corresponding subcategories.

\subsubsection*{A.2.1 ICD-11 Classification Prompt}
\begin{tcolorbox}[colback=gray!5!white,colframe=gray!55!white,before upper={\raggedright},title=ICD-11 Classification Prompt]
You are a medical classification expert. Analyze the given medical question and classify it according to ICD-11 guidelines.\\
\vspace{1em}
Follow this reasoning process:\\
1. First, analyze the question to determine which major category best fits based on ICD-11 classification\\
2. Then, from that specific category's subcategories, select the most appropriate diagnosis\\
\vspace{1em}
Return ONLY the raw JSON object, without any markdown formatting or other explanatory text. The JSON object should look like this:
\vspace{0.5em}
\begin{spacing}{1.0}
\begin{lstlisting}[breaklines=true, basicstyle=\ttfamily\normalsize]
{
    "major_category": "[Selected major category]",
    "specific_diagnosis": "[Selected specific diagnosis from the corresponding subcategory]"
}
\end{lstlisting}
\end{spacing}
\vspace{0.5em}
Question: [{question}]
\end{tcolorbox}

\subsubsection*{A.2.2 Medical Category Classification Prompt}

\begin{tcolorbox}[colback=gray!5!white,colframe=gray!55!white,before upper={\raggedright},title=Medical Category Classification Prompt]
Given the following medical question, classify it into ONE of the following three categories:\\
\vspace{1em}

- Basic sciences and pathophysiology\\
- Clinical knowledge and disease management\\
- Clinical management and patient care decision-making\\
\vspace{1em}
Analyze the question and determine which category it best fits.
\vspace{1em}
Question: <question>

Return ONLY the raw JSON object, without any markdown formatting or other explanatory text. The JSON object should look like this:
\vspace{0.5em}
\begin{spacing}{1.0}
\begin{lstlisting}[breaklines=true, basicstyle=\ttfamily\normalsize]
{
    "category": "[Selected category]"
}
\end{lstlisting}
\end{spacing}
\end{tcolorbox}

% \begin{tcolorbox}[
%     colback=gray!5!white,
%     colframe=gray!55!white,
%     before upper={\raggedright},
%     title=Supplementary Information Tables,
%     breakable]
% You are a psychiatric diagnostic specialist with extensive knowledge of ICD-11 classification systems. Carefully analyze the following psychiatric question and classify it using a two-step hierarchical approach.

% \vspace{0.5em}

% \textbf{STEP 1:} Identify the \textbf{major\_category} from these main ICD-11 categories:\textbf{LIST\_OF\_ICD11}

% \vspace{0.5em}
% \textbf{STEP 2:} Based on the \textbf{major\_category} identified in Step 1, select the most specific diagnosis from the corresponding ICD-11 subcategories.\\

% \vspace{0.5em}
% \begin{center}
% \fbox{%
%   \parbox{0.6\linewidth}{\centering
%     \vspace{0.5em}
%     IF \textbf{major\_category} in \textbf{LIST\_OF\_ICD11}:\\[0.5em]
%     \textbf{SUB\_List} = MAP(\textbf{major\_category})\\[0.5em]
%     SELECT the most matched category in \textbf{SUB\_List}\\[0.5em]
%   }%
% }
% \end{center}
% \vspace{0.5em}
% \textbf{Question: "<QUESTION FROM DATASET>"}
% \end{tcolorbox}

%---------------------------------------A.3------------------------------------------%
\newpage
\subsection*{A.3 Evaluation Prompts}
\vspace{0.5em}
The following prompts are used to evaluate the model's performance on psychiatric multiple-choice questions. The model is instructed to respond as a professional psychiatrist and provide only the letter corresponding to the correct answer.

\subsubsection*{A.3.1 Evaluation Prompt for Non-Reasoning Model}
\begin{tcolorbox}[colback=gray!5!white,colframe=gray!55!white,title=Psychiatric Evaluation Prompt]
You are a professional psychiatrist with extensive clinical diagnosis and treatment experience. Based on your expertise, carefully read the following psychiatric question and select the most accurate answer.
\vspace{0.5em}
Please respond ONLY with the letter (A, B, C, D), without explanation.

\vspace{0.5em}

Question: \{question\}
\vspace{0.5em}\\
A. \{Option A\} \\
B. \{Option B\} \\
C. \{Option C\} \\
D. \{Option D\}
\end{tcolorbox}

\subsubsection*{A.3.2 Evaluation Prompt for Reasoning Model}

\begin{tcolorbox}[colback=gray!5!white,colframe=gray!55!white,title=Reasoning Psychiatric Evaluation Prompt]
You are a medical specialist with extensive knowledge in Psychiatry. Carefully analyze the following question and select the most appropriate answer.

\vspace{0.5em}

Question: \{question\}
\vspace{0.5em}

A. \{Option A\}\\
B. \{Option B\}\\
C. \{Option C\}\\
D. \{Option D\}\\

\vspace{0.5em}

Provide ONLY the letter (A, B, C, D) corresponding to the best answer. NO OTHER EXPLANATION.
Example Output Format: A OR B OR C OR D (Exactly one letter, no punctuation, no additional text)
\end{tcolorbox}
